# Supplementary material for: Toward End-to-End MLOps Tools Map: A Preliminary Study based on a Multivocal Literature Review
Source: arXiv:2304.03254 source file (2023-04-06)
Supplement: Supplementary file 1 [file Appendix_A.tex]

\section*{Primary Studies}

\begin{enumerate}[\footnotesize, label={[PS}{\arabic*]}]
\smallskip \item	
F. Melchor, R. Rodriguez-Echeverria, J.M. Conejero, Á.E. Prieto, J.D. Gutiérrez,		&"	A Model-Driven Approach for Systematic Reproducibility and Replicability of Data Science Projects	",&		Lecture Notes in Computer Science (including subseries Lecture Notes in Artificial Intelligence and Lecture Notes in Bioinformatics),&		2022.
\smallskip \item	
H. Khalajzadeh, M. Abdelrazek, J. Grundy, J. Hosking and Q. He,		&"	A Survey of Current End-user Data Analytics Tool Support	",&		International Congress on Big Data,&		2018.
\smallskip \item
M.N. Chowdary, B. Sankeerth, C.K. Chowdary and M. Gupta,		&"	Accelerating the Machine Learning Model Deployment using MLOps	",&		Journal of Physics: Conference Series,&		2022.
\smallskip \item	
S. Laato, T. Birkstedt, M. Mantymaki, M. Minkkinen and T. Mikkonen, 		&"	AI Governance in the System Development Life Cycle: Insights on Responsible Machine Learning Engineering	",&		Proceedings - 1st International Conference on AI Engineering - Software Engineering for AI, CAIN 2022,&		2022.
\smallskip \item	
D. Nigenda, Z. Karnin, M. B. Zafar, R. Ramesha, A. Tan, M. Donini and K. Kenthapadi,		&"	Amazon SageMaker Model Monitor: A System for Real-Time Insights into Deployed Machine Learning Models	",&		KDD 2022,&		2022.
\smallskip \item	
H. Khalajzadeh, A. Simmons, M. Abdelrazek, J. Grundy, J. Hosking and Q. He,		&"	An end-to-end model-based approach to support big data analytics development	",&		Journal of Visual Languages and Computign,&		2019.
\smallskip \item
K.-H. Chen, H.-P. Su, W.-C. Chuang, H.-C. Hsiao, W. Tan, Z. Tang, X. Liu, Y. Liang, W.-C. Lo, W. Ji, B. Hsu, K. Hu, H.Y. Jian, Q. Zhou and C.-M. Wang,		&"	Apache submarine: a unified machine learning platform made simple	",&		Proceedings of the 2nd European Workshop on Machine Learning and Systems,&		2022.
\smallskip \item
O. Berezsky, O. Pitsun, G. Melnyk, Y. Batko, B. Derysh and P. Liashchynskyi,		&"	Application Of MLOps Practices For Biomedical Image Classification	",&		CEUR Workshop Proceedings,&		2022.
\smallskip \item
P. Ruf, C. Reich and D. Ould-Abdeslam,		&"	Aspects of Module Placement in Machine Learning Operations for Cyber Physical Systems	",&		2022 11th Mediterranean Conference on Embedded Computing, MECO 2022,&		2022.
\smallskip \item
C. Vuppalapati, A. Ilapakurti, K. Chillara, S. Kedari and V. Mamidi,		&"	Automating Tiny ML Intelligent Sensors DevOPS Using Microsoft Azure	",&		Proceedings - 2020 IEEE International Conference on Big Data, Big Data 2020,&		2020.
\smallskip \item
L. Cardoso Silva, F. Rezende Zagatti, B. Silva Sette, L. Nildaimon Dos Santos Silva, D. Lucredio, D. Furtado Silva and H. De Medeiros Caseli,		&"	Benchmarking Machine Learning Solutions in Production	",&		Proceedings - 19th IEEE International Conference on Machine Learning and Applications, ICMLA 2020,&		2020.
\smallskip \item
Y. Liu, Z. Ling, B. Huo, B. Wang, T. Chen and E. Mouine, 		&"	Building A Platform for Machine Learning Operations from Open Source Frameworks	",&		IFAC-PapersOnLine,&		2020.
\smallskip \item
A. Paleyes, R.-G. Urma and N. D. Lawrence,		&"	Challenges in Deploying Machine Learning: A Survey of Case Studies	",&		ACM Computing Surveys 55.6,&		2022.
\smallskip \item
S.E. Whang, Y. Roh, H. Song and J.-G. Lee,		&"	Data collection and quality challenges in deep learning: a data-centric AI perspective	",&		VLDB Journal,&		2023.
\smallskip \item
P. Ruf, M. Madan, C. Reich and D. Ould-Abdeslam, 		&"	Demystifying mlops and presenting a recipe for the selection of open-source tools	",&		Applied Sciences (Switzerland),&		2021.
\smallskip \item
D. Yang, D. Wang, D. Yang, Q. Dong, Y. Wang, H. Zhou and H. Daocheng,		&"	DevOps in practice for education management information system at ECNU	",&		Procedia Computer Science,&		2020.
\smallskip \item
N. Baumann, E. Kusmenko, J. Ritz, B. Rumpe and M.B. Weber,		&"	Dynamic data management for continuous retraining	",&		Proceedings - ACM/IEEE 25th International Conference on Model Driven Engineering Languages and Systems, MODELS 2022: Companion Proceedings,&		2022.
\smallskip \item
H. Zahid, T. Mahmood and N. Ikram,		&"	Enhancing Dependability in Big Data Analytics Enterprise Pipelines	",&		International Conference on Security, Privacy and Anonymity in Computation, Communication and Storage,&		2018.
\smallskip \item
T. Mahapatra and S.N. Banoo,		&"	Flow-based programming for machine learning	",&		Future Internet,&		2022.
\smallskip \item
A. Capizzi, S. Distefano and M. Mazzara,		&"	From DevOps to DevDataOps: Data Management in DevOps Processes	",&		Lecture Notes in Computer Science (including subseries Lecture Notes in Artificial Intelligence and Lecture Notes in Bioinformatics),&		2020.
\smallskip \item
T. Hegeman, M. Jansen, A. Iosup and A. Trivedi,		&"	GradeML: Towards holistic performance analysis for machine learning workflows	",&		ICPE 2021 - Companion of the ACM/SPEC International Conference on Performance Engineering,&		2021.
\smallskip \item
M. Langenkamp and D.N. Yue,		&"	How Open Source Machine Learning Software Shapes AI	",&		AIES 2022 - Proceedings of the 2022 AAAI/ACM Conference on AI, Ethics, and Society,&		2022.
\smallskip \item
L. Rosa, T. Cruz, M.B.D. Freitas, P. Quitério, J. Henriques, F. Caldeira, E. Monteiro and P. Simões,		&"	Intrusion and anomaly detection for the next-generation of industrial automation and control systems	",&		Future Generation Computer Systems,&		2021.
\smallskip \item
D.R. Niranjan and Mohana,		&"	Jenkins Pipelines: A Novel Approach to Machine Learning Operations (MLOps)	",&		International Conference on Edge Computing and Applications, ICECAA 2022 - Proceedings,&		2022.
\smallskip \item
G. Zarate, R. Minon, J. Diaz-De-Arcaya and A.I. Torre-Bastida,		&"	K2E: Building MLOps Environments for Governing Data and Models Catalogues while Tracking Versions	",&		2022 IEEE 19th International Conference on Software Architecture Companion, ICSA-C 2022,&		2022.
\smallskip \item
C. Martín, P. Langendoerfer, P.S. Zarrin, M. Díaz and B. Rubio,		&"	Kafka-ML: Connecting the data stream with ML/AI frameworks	",&		Future Generation Computer Systems,&		2022.
\smallskip \item
I.L. Markov, H. Wang, N.S. Kasturi, S. Singh, M.R. Garrard, Y. Huang, S.W.C. Yuen, S. Tran, Z. Wang, I. Glotov, T. Gupta, P. Chen, B. Huang, X. Xie, M. Belkin, S. Uryasev, S. Howie, E. Bakshy and N. Zhou,		&"	Looper: An End-to-End ML Platform for Product Decisions	",&		Proceedings of the ACM SIGKDD International Conference on Knowledge Discovery and Data Mining,&		2022.
\smallskip \item
P. Tomaszewski, S. Yu, M. Borg and J. Ronnols,		&"	Machine Learning-Assisted Analysis of Small Angle X-ray Scattering	",&		Proceedings of the 2021 Swedish Workshop on Data Science, SweDS 2021,&		2021.
\smallskip \item
B. Derakhshan, A. Rezaei Mahdiraji, Z. Kaoudi, T. Rabl and V. Markl,		&"	Materialization and Reuse Optimizations for Production Data Science Pipelines	",&		Proceedings of the ACM SIGMOD International Conference on Management of Data,&		2022.
\smallskip \item
A. Molner Domenech and A. Guillén,		&"	Ml-experiment: A Python framework for reproducible data science	",&		Journal of Physics: Conference Series,&		2020.
\smallskip \item
G. Symeonidis, E. Nerantzis, A. Kazakis and G.A. Papakostas,		&"	MLOps - Definitions, Tools and Challenges	",&		2022 IEEE 12th Annual Computing and Communication Workshop and Conference, CCWC 2022,&		2022.
\smallskip \item
M. Testi, M. Ballabio, E. Frontoni, G. Iannello, S. Moccia, P.Soda and G. Vessio,		&"	MLOps: A Taxonomy and a Methodology	",&		IEEE Access,&		2022.
\smallskip \item
R. Minon, J. Diaz-De-Arcaya, A.I. Torre-Bastida, G. Zarate and A. Moreno-Fernandez-De-Leceta,		&"	MLPacker: A Unified Software Tool for Packaging and Deploying Atomic and Distributed Analytic Pipelines	",&		2022 7th International Conference on Smart and Sustainable Technologies, SpliTech 2022,&		2022.
\smallskip \item
A.T. Njomou, A. Johanne Bifona Africa, B. Adams and M. Fokaefs,		&"	MSR4ML: Reconstructing Artifact Traceability in Machine Learning Repositories	",&		Proceedings - 2021 IEEE International Conference on Software Analysis, Evolution and Reengineering, SANER 2021,&		2021.
\smallskip \item
H. Lee, Y. Jang, J. Song and H. Yeon,		&"	O-RAN AI/ML Workflow Implementation of Personalized Network Optimization via Reinforcement Learning	",&		2021 IEEE Globecom Workshops, GC Wkshps 2021 - Proceedings,&		2021.
\smallskip \item
S. Garg, P. Pundir, G. Rathee, P.K. Gupta, S. Garg and S. Ahlawat,		&"	On Continuous Integration / Continuous Delivery for Automated Deployment of Machine Learning Models using MLOps	",&		Proceedings - 2021 IEEE 4th International Conference on Artificial Intelligence and Knowledge Engineering, AIKE 2021,&		2021.
\smallskip \item
A. Barrak, E.E. Eghan and B. Adams,		&"	On the Co-evolution of ML Pipelines and Source Code - Empirical Study of DVC Projects	",&		Proceedings - 2021 IEEE International Conference on Software Analysis, Evolution and Reengineering, SANER 2021,&		2021.
\smallskip \item
J. Díaz-de-Arcaya, A.I. Torre-Bastida, R. Miñón and A. Almeida,		&"	Orfeon: An AIOps framework for the goal-driven operationalization of distributed analytical pipelines	",&		Future Generation Computer Systems,&		2023.
\smallskip \item
R. Miñón, J. Diaz-De-arcaya, A.I. Torre-Bastida and P. Hartlieb,		&"	Pangea: An MLOps Tool for Automatically Generating Infrastructure and Deploying Analytic Pipelines in Edge, Fog and Cloud Layers	",&		Sensors,&		2022.
\smallskip \item
G. Quattrocchi and D.A. Tamburri,		&"	Predictive maintenance of infrastructure code using “fluid” datasets: An exploratory study on Ansible defect proneness	",&		Journal of Software: Evolution and Process,&		2022.
\smallskip \item
N. Rauschmayr, S. Kama, M. Kim, M. Choi and K. Kenthapadi,		&"	Profiling Deep Learning Workloads at Scale using Amazon SageMaker	",&		KDD 2022,&		2022.
\smallskip \item
E. Zeydan and J. Mangues-Bafalluy,		&"	Recent Advances in Data Engineering for Networking	",&		IEEE Access,&		2022.
\smallskip \item
Hagos D.H., Kakantousis T., Sheikholeslami S., Wang T., Vlassov V., Payberah A.H., Meister M., Andersson R., Dowling J.		&"	Scalable Artificial Intelligence for Earth Observation Data Using Hopsworks	",&		Remote Sensing,&		2022.
\smallskip \item
Y. D. Dessalk, N. Nikolov, M. Matskin, A. Soylu and D. Roman,		&"	Scalable Execution of Big Data Workflows using Software Containers	",&		Proceedings of the 12th International Conference on Management of Digital EcoSystems,&		2020.
\smallskip \item
D. Patel, S. Shrivastava, W. Gifford, S. Siegel, J. Kalagnanam and C. Reddy,		&"	Smart-ML: A System for Machine Learning Model Exploration using Pipeline Graph	",&		Proceedings - 2020 IEEE International Conference on Big Data, Big Data 2020,&		2020.
\smallskip \item
M. Openja, F. Majidi, F. Khomh, B. Chembakottu and H. Li,		&"	Studying the Practices of Deploying Machine Learning Projects on Docker	",&		ACM International Conference Proceeding Series,&		2022.
\smallskip \item
D.A. Tamburri,		&"	Sustainable MLOps: Trends and Challenges	",&		Proceedings - 2020 22nd International Symposium on Symbolic and Numeric Algorithms for Scientific Computing, SYNASC 2020,&		2020.
\smallskip \item
O. Spjuth, J. Frid and A.  Hellander,		&"	The machine learning life cycle and the cloud: implications for drug discovery	",&		Expert Opinion on Drug Discovery,&		2021.
\smallskip \item
Y. Zhou, Y. Yu and B. Ding,		&"	Towards MLOps: A Case Study of ML Pipeline Platform	",&		Proceedings - 2020 International Conference on Artificial Intelligence and Computer Engineering, ICAICE 2020,&		2020.
\smallskip \item
W. Wu and C. Zhang		&"	Towards understanding end-to-end learning in the context of data: Machine learning dancing over semirings \& Codd's table	",&		Proceedings of the 5th Workshop on Data Management for End-To-End Machine Learning, DEEM 2021 - In conjunction with the 2021 ACM SIGMOD/PODS Conference,&		2021.
\smallskip \item
B. Benni, M. Blay-Fornarino, S. Mosser, F. Precisio and G. Jungbluth,		&"	When DevOps meets meta-learning: a portfolio to rule them all	",&		2019 ACM/IEEE 22nd International Conference on Model Driven Engineering Languages and Systems Companion (MODELS-C),&		2021.
\smallskip \item
Lago72	,	&"	\#Kubeflow vs \#MLflow – Which \#MLOps tool should you use. Kubeflow provides components for each stage in the \#ML lifecycle, including exploration, training and deployment. https://t.co/D5Zxu3Mv9x v/ @Analyticsindiam   \#BigData \#Analytics \#DataScience \#AI \#IoT \#IIoT \#CloudComputing https://t.co/zEvDdhpf7p	",&	\url{	https://twitter.com/Lago72/status/1501982718745354243	},&		2022.
\smallskip \item
DanielBookmarks	,	&"	\#MLOps became a hot buzzword. It sparked a gold rush for software vendors, so it's hard to choose the best tool for your needs. Save time, learn about \#VertexAI (MLOps platforms for entire \#AI/\#ML \#workflow on \#GoogleCloud) at the next \#ServerlessTO meetup https://t.co/7qWsJYPFT4	",&	\url{	https://twitter.com/DanielBookmarks/status/1459178976803491884	},&		2021.
\smallskip \item
datacouch\textunderscore io	,	&"	\#MLOps for Python models using \#Azure \#MachineLearning! The architecture shows how to implement \#continuousintegration, \#continuousdelivery, and retraining pipeline for an \#AI application using Azure DevOps and Azure ML. Let's Explore... Source: https://t.co/qEu0J6O3oY https://t.co/uQwAUp7YdC	",&	\url{	https://twitter.com/datacouch_io/status/1407662236701585409	},&		2021.
\smallskip \item
L. Lancaster	,	&"	\#Observability: It's Time to Automate the Observer! Zebrium CTO Larry Lancaster writes about \#application \#monitoring trends \&amp; the importance of delivering a platform-agnostic, out-of-the-box solution to automate troubleshooting. https://t.co/Bm4lT7gc48 \#devops \#sre \#apm \#MLOps	",&	\url{	https://twitter.com/ZebriumAI/status/1537095861989126146	},&		2022.
\smallskip \item
P. Sharma	,	&"	10 Best MLOps Tools in 2022 - Pratik Sharma	",&	\url{	https://www.pratikdsharma.com/10-best-mlops-tools-in-2022/	},&		2022.
\smallskip \item
M. Heller	,	&"	10 MLops platforms to manage the machine learning lifecycle	",&	\url{	https://www.infoworld.com/article/3572442/10-mlops-platforms-to-manage-the-machine-learning-lifecycle.html	},&		2020.
\smallskip \item
A. A. Awan	,	&"	17 Top MLOps Tools You Need to Know - DataCamp	",&	\url{	https://www.datacamp.com/blog/top-mlops-tools	},&		2022.
\smallskip \item
NimbleBoxAI	,	&"	2. As an MLOps tool @MLflow, caters to your entire Machine Learning pipeline by providing tools that include modularity and automation in experimentation, reproducibility, and much more!️	",&	\url{	https://twitter.com/NimbleBoxAI/status/1493120712214986754	},&		2022.
\smallskip \item
dkedar7	,	&"	2. Workflow orchestration:  Tools that allow us to define, manage and schedule DAGs (Directed Acyclic Graphs)   Open-source tools are common – battle-tested tools like @ApacheAirflow, Argo.   Chances are that an open-source tool suits your MLOps better than any in-house tool	",&	\url{	https://twitter.com/dkedar7/status/1415118827432595460	},&		2021.
\smallskip \item
u/mgalarny	,	&"	5 considerations for Deploying Machine Learning Models in Production – what did I miss?	",&	\url{	https://www.reddit.com/r/MachineLearning/comments/qz3qtv/d_5_considerations_for_deploying_machine_learning/	},&		2021.
\smallskip \item
u/TirendazAcademy	,	&"	7 Best Machine Learning Experiment Logging Tools in 2022	",&	\url{	https://www.reddit.com/r/learnmachinelearning/comments/xnk3kt/7_best_machine_learning_experiment_logging_tools/	},&		2022.
\smallskip \item
Veritone	,	&"	9 Helpful MLOps Tools You Should Consider Using Right Now	",&	\url{	https://www.veritone.com/blog/9-helpful-mlops-tools-you-should-consider-using-right-now/	},&		2022.
\smallskip \item
kelvins	,	&"	A curated list of awesome MLOps tools - GitHub	",&	\url{	https://github.com/kelvins/awesome-mlops	},&	Accessed 2023.
\smallskip \item
S.Pierre	,	&"	A Survey of the Top Three MLOps tools - Towards Data Science	",&	\url{	https://towardsdatascience.com/a-survey-of-the-top-three-mlops-tools-1694688648c5	},&		2022.
\smallskip \item
Accellario	,	&"	Accelario DataOps Platform - Accelario	",&	\url{	https://accelario.com/products/accelario-dataops-platform/	},&	Accessed 2023.
\smallskip \item
blaizeinc	,	&"	AI Studio - transforming productivity for faster ROI of edge AI deployments. Read more about the unveiling of their open and code-free software platform. https://t.co/S4GEw9CIPm	",&	\url{	https://twitter.com/blaizeinc/status/1339588931688357891	},&		2020.
\smallskip \item
M. Schmitt	,	&"	Airflow vs. Luigi vs. Argo vs. MLFlow vs. KubeFlow	",&	\url{	https://towardsdatascience.com/airflow-vs-luigi-vs-argo-vs-mlflow-vs-kubeflow-b3785dd1ed0c	},&		2020.
\smallskip \item
Shyam BV	,	&"	Airflow Vs. Prefect — Workflow management for Data projects	",&	\url{	https://medium.com/towards-data-science/airflow-vs-prefect-workflow-management-for-data-projects-5d1a0c80f2e3	},&		2021.
\smallskip \item
enjoydana	,	&"	Are you a guy that supports IA teams? Here, Bodywork. It's an MLOPs pipeline tool. \#Kubernetes \#MLOps \#devops \#IA \#github	",&	\url{	https://twitter.com/enjoydana/status/1553007791148785665	},&		2022.
\smallskip \item
LabelStudioHQ	,	&"	Are you missing an important piece of your data annotation workflow? Label Studio is an open-source tool that can help fill the gaps.  Privacy by default.  Security baked in.  Runs on your infra.  \#MLOps \#MachineLearning https://t.co/ubTWSqEqdg	",&	\url{	https://twitter.com/LabelStudioHQ/status/1263169100337070082	},&		2020.
\smallskip \item
mafqcm	,	&"	As per the page "Dataiku Data Science Studio is a good tool for 'citizen' data scientists. It offers business users data connectivity, charts, and simple analysis tools. Domino is a platform for expert data scientists." https://t.co/wqGegB9PBe	",&	\url{	https://twitter.com/mafqcm/status/1614945663288233994	},&		2023.
\smallskip \item
Aporia team	,	&"	Best Data Versioning Tools for MLOps | Aporia Blog	",&	\url{	https://www.aporia.com/blog/best-data-version-tools-for-mlops-2021/	},&	Accessed 2023.
\smallskip \item
SourceForge	,	&"	Best MLOps Platforms and Tools of 2023 - SourceForge	",&	\url{	https://sourceforge.net/software/mlops/	},&	Accessed 2023.
\smallskip \item
K. Kimachia	,	&"	Best MLOps Tools \& Platforms 2022 | ITBE - IT Business Edge	",&	\url{	https://www.itbusinessedge.com/development/mlops-tools/	},&		2022.
\smallskip \item
S. Hiter	,	&"	Best MLOps Tools \& Platforms for 2022 | CIO Insight	",&	\url{	https://www.cioinsight.com/it-strategy/best-mlops-tools/	},&		2022.
\smallskip \item
T. Shridar	,	&"	Best MLOps Tools: What to Look for and How to Evaluate Them	",&	\url{	https://nimblebox.ai/blog/mlops-tools	},&		2022.
\smallskip \item
u/xela-sedinnaoi	,	&"	Bodywork - ML pipelines on Kubernetes	",&	\url{	https://www.reddit.com/r/mlops/comments/vrrs1z/bodywork_ml_pipelines_on_kubernetes/	},&		2022.
\smallskip \item
K8sArchitect	,	&"	Bodywork is a MLOps tool which can be used to deploy machine learning model pipelines to Kubernetes. It is a more lightweight and simpler alternative when compared to tools like KubeFlow ➤ https://t.co/ZOWFdwXUKd https://t.co/ob25B6tEj8	",&	\url{	https://twitter.com/K8sArchitect/status/1552642533687271426	},&		2022.
\smallskip \item
Samhita Alla	,	&"	Build Indestructible Pipelines With Flyte	",&	\url{	https://medium.com/union-ai/build-indestructible-pipelines-with-flyte-5ef9348d4670	},&		2021.
\smallskip \item
F. Pachinger	,	&"	Building a ML Pipeline from Scratch with Kubeflow – MLOps ...	",&	\url{	https://blogs.cisco.com/developer/machinelearningops03	},&		2022.
\smallskip \item
PolyaxonAI	,	&"	Check this \#Ansible Playbook that enables to automate Polyaxon's \#AIOps/\#MLOps Platform by \#Dell Technologies and the \#Omnia tool  https://t.co/dzD7LOs1k5	",&	\url{	https://twitter.com/PolyaxonAI/status/1426888032599351297	},&		2021.
\smallskip \item
ClearML	,	&"	ClearML: MLOps for Data Scientists, ML Engineers, and DevOps	",&	\url{	https://clear.ml/	},&	Accessed 2023.
\smallskip \item
CodeProject	,	&"	CodeProject - For those who code	",&	\url{	https://www.codeproject.com/	},&	Accessed 2023.
\smallskip \item
M. Schmitt	,	&"	Comparing managed machine learning platforms	",&	\url{	https://medium.com/towards-data-science/dataiku-vs-alteryx-vs-sagemaker-vs-datarobot-vs-databricks-b3870bd34813	},&		2020.
\smallskip \item
J. Teichmann	,	&"	Complete Data Science Project Template with Mlflow for Non-Dummies.	",&	\url{	https://towardsdatascience.com/complete-data-science-project-template-with-mlflow-for-non-dummies-d082165559eb	},&		2019.
\smallskip \item
Composable AI	,	&"	Composable Analytics | Intelligent DataOps. Enterprise AI ...	",&	\url{	https://composable.ai/	},&	Accessed on	2023.
\smallskip \item
M. Cerruti	,	&"	Continuous integration and -deployment with GitHub, CircleCI and Kubernetes in Azure	",&	\url{	https://medium.com/@aevitas/continuous-integration-and-deployment-with-github-circleci-and-kubernetes-50405716de7c	},&		2018.
\smallskip \item
Django Stars	,	&"	Continuous Integration. CircleCI vs Travis CI vs Jenkins	",&	\url{	https://medium.com/hackernoon/continuous-integration-circleci-vs-travis-ci-vs-jenkins-41a1c2bd95f5	},&		2017.
\smallskip \item
zenml\textunderscore io	,	&"	Continuously train and deploy your machine learning models AND integrate your pipeline into a data application with @streamlit in minutes!  What an amazing showcase of how ZenML is bringing different tooling worlds together!  \#opensource \#MLOps https://t.co/h7UorQD0ba	",&	\url{	https://twitter.com/zenml_io/status/1517158235819573251	},&		2022.
\smallskip \item
u/datasnow	,	&"	Critique/help with the MLOps plan for a small DS team	",&	\url{	https://www.reddit.com/r/datascience/comments/g8ojeg/critiquehelp_with_the_mlops_plan_for_a_small_ds/	},&		2020.
\smallskip \item
DiogenesWallis	,	&"	D75 \#66daysofdata Today I made an ETL pipeline using airflow. I could visualize the DAG structure in the airflow GUI and see the time consumed by each task (node). I also discovered that airflow can be used as MLOps tool. Kubeflow or Airflow? Which do you pick?	",&	\url{	https://twitter.com/DiogenesWallis/status/1529647262883782656	},&		2022.
\smallskip \item
Khuyen Tran	,	&"	DagsHub: a GitHub Supplement for Data Scientists and ML Engineers	",&	\url{	https://medium.com/towards-data-science/dagshub-a-github-supplement-for-data-scientists-and-ml-engineers-9ecaf49cc505	},&		2022.
\smallskip \item
Pachyderm	,	&"	Data + The MLOps Lifecycle - Pachyderm	",&	\url{	https://www.pachyderm.com/solutions/mlops/	},&	Accessed 2023.
\smallskip \item
Data Version Control	,	&"	Data Version Control · DVC	",&	\url{	https://dvc.org/	},&	Accessed 2023.
\smallskip \item
u/thumbsdrivesmecrazy	,	&"	Data Version Control (DVC) 1.0 release: Git for data with new features for MLOps and collaboration on ML projects	",&	\url{	https://www.reddit.com/r/codetogether/comments/hee1kj/data_version_control_dvc_10_release_git_for_data/	},&		2020.
\smallskip \item
hksokhi	,	&"	Data versioning and data management are core components of \#MLOps and \#AI platform. Join Data Engineering Melbourne Meetup(online) to hear from the  creator of open-source tool Data Version Control - \#DVC , Dmitry Petrov ,talk abou…https://t.co/9tZzjuHO2g https://t.co/SSkSdswXt7	",&	\url{	https://twitter.com/hksokhi/status/1308226957767774209	},&		2020.
\smallskip \item
DataKitchen	,	&"	DataKitchen: DataOps Observability and Automation Software	",&	\url{	https://datakitchen.io/	},&		2020.
\smallskip \item
IBM	,	&"	DataOps Platform Solutions - IBM	",&	\url{	https://www.ibm.com/dataops	},&	Accessed 2023.
\smallskip \item
P. Nguyen	,	&"	DataOps: Framework, Tools and Everything In Between	",&	\url{	https://www.holistics.io/blog/dataops-framework-tools/	},&		2022.
\smallskip \item
Datatron	,	&"	Datatron: MLOps Platform with Scale and Security	",&	\url{	https://datatron.com/	},&	Accessed 2023.
\smallskip \item
PathikGhugare	,	&"	Day 14, \#60daysofcode After learning about Experiment tracking and Model registry concepts of \#mlops, I started off with the 3rd week of \#mlopszoomcamp which teaches about "Workflow Orchestration" Also, learnt about "Negative Engineering" and got introduced to tool @PrefectIO	",&	\url{	https://twitter.com/PathikGhugare/status/1541126974424641536	},&		2022.
\smallskip \item
dbt	,	&"	dbt - Transform data in your warehouse	",&	\url{	https://www.getdbt.com/	},&	Accessed 2023.
\smallskip \item
u/modzykirsten	,	&"	Deploy, run, and monitor ML/AI models for free with Modzy Basic+	",&	\url{	https://www.reddit.com/r/developers/comments/vibabs/deploy_run_and_monitor_mlai_models_for_free_with/	},&		2022.
\smallskip \item
valohaiai	,	&"	Did you know that the Valohai platform is tool agnostic? You can use any framework in any programming language and Valohai takes care of the \#MLOps for you. https://t.co/TPQPKorGRM \#Keras \#TensorFlow \#Darknet \#PyTorch \#Torch \#Caffe \#NumPy \#DL4J \#Python \#R etc. https://t.co/pxmbVzuh5o	",&	\url{	https://twitter.com/valohaiai/status/1166879135593107457	},&		2019.
\smallskip \item
valohaiai	,	&"	Did you know that you can do distributed learning with Valohai?  Having this feature is not only a nice-to-have flex for us as an \#MLOps platform but a valuable tool for your business: https://t.co/UTZSraXjJg	",&	\url{	https://twitter.com/valohaiai/status/1552911802446618624	},&		2022.
\smallskip \item
aniketmaurya	,	&"	Do you know that with Lightning AI you can build a complete end-to-end machine learning pipeline? You can build a machine learning training, and deployment pipeline and connect your favorite MLOps tool to monitor your model in production. 1/2	",&	\url{	https://twitter.com/aniketmaurya/status/1603693201985978368	},&		2022.
\smallskip \item
Domino Data Lab	,	&"	Domino Enterprise MLOps Platform	",&	\url{	https://www.dominodatalab.com/product/domino-enterprise-mlops-platform	},&	Accessed 2023.
\smallskip \item
M. Ali	,	&"	Easy MLOps with PyCaret + MLflow	",&	\url{	https://towardsdatascience.com/easy-mlops-with-pycaret-mlflow-7fbcbf1e38c6	},&		2021.
\smallskip \item
leomerle5	,	&"	Edge AI deployments today are complicated by a lack of tools for application development and MLOps. @blaizeinc AI Studio was born to address the complete end-to-end edge AI operational workflow.	",&	\url{	https://twitter.com/leomerle5/status/1339684842942820353	},&		2020.
\smallskip \item
R. Nakod	,	&"	Efficient MLOps through AI application containerization	",&	\url{	https://www.embedded.com/efficient-mlops-through-ai-application-containerization/	},&		2022.
\smallskip \item
Harsha V	,	&"	End to End MLOps using MLflow	",&	\url{	https://www.clearpeaks.com/end-to-end-mlops-using-mlflow/	},&		2022.
\smallskip \item
R. Dawson and D. Sato	,	&"	Evaluating MLOps Platforms - Thoughtworks	",&	\url{	https://www.thoughtworks.com/content/dam/thoughtworks/documents/whitepaper/tw_whitepaper_guide_to_evaluating_mlops_platforms_2021.pdf	},&		2021.
\smallskip \item
u/obsezer	,	&"	Fast-Kubeflow: Kubeflow Tutorial, Sample Usage Scenarios (Howto: Hands-on LAB)	",&	\url{	https://www.reddit.com/r/mlops/comments/103bm9p/fastkubeflow_kubeflow_tutorial_sample_usage/	},&		2023.
\smallskip \item
PatchenNoelke	,	&"	For a little more detail...we build a Framework that can serve as a planning guide for ML Ops. Details out: 1. The Workflow, 2. Technology layers, 3. Algorithm to Application journey. https://t.co/bTtkX2bYwh	",&	\url{	https://twitter.com/PatchenNoelke/status/1274016849408081920	},&		2020.
\smallskip \item
neptune\textunderscore ai	,	&"	For organizations that want an "all-in-one" \#MLOps solution, Azure ML is a great tool. But what if you don’t need such a complex platform?  Here are some alternative tools for tasks like experiment tracking, model management, model deployment, and more. https://t.co/FmlogmZ793	",&	\url{	https://twitter.com/neptune_ai/status/1458486364811505666	},&		2021.
\smallskip \item
Stefano Bosisio	,	&"	From Dev to Deployment: An End to End Sentiment Classifier App with MLflow, SageMaker, and Streamlit	",&	\url{	https://medium.com/towards-data-science/from-dev-to-deployment-an-end-to-end-sentiment-classifier-app-with-mlflow-sagemaker-and-119043ea4203	},&		2022.
\smallskip \item
JeremiahKamama	,	&"	Google has now entered the MLOps arena with Vertex AI. Google Cloud unveils Vertex AI, one platform, every ML tool you need https://t.co/TaUIDPuUSe	",&	\url{	https://twitter.com/JeremiahKamama/status/1394904015419367425	},&		2021.
\smallskip \item
Paperspace	,	&"	Gradient MLOps Platform - Paperspace	",&	\url{	https://www.paperspace.com/gradient	},&	Accessed 2023.
\smallskip \item
santaferraro	,	&"	Great briefing with StreamSets Inc. this afternoon. I love the flexibility StreamSets Transformer and the way it opens up data pipeline management to a broader set of users. I got to see the MLOps application in pipelines and now my mind is going crazy tr…https://t.co/W5eivKixnD	",&	\url{	https://twitter.com/santaferraro/status/1230613416957612032	},&		2020.
\smallskip \item
chezou	,	&"	Great ML Ops tool from Lyft covering lineage, workflow as Python DSL/Introducing Flyte: A Cloud Native Machine Learning and Data Processing Platform https://t.co/05GG3SODGl	",&	\url{	https://twitter.com/chezou/status/1214784698641084416	},&		2020.
\smallskip \item
u/rom1001	,	&"	Help on understanding mlops tools.	",&	\url{	https://www.reddit.com/r/mlops/comments/pzzqqu/help_on_understanding_mlops_tools/	},&		2021.
\smallskip \item
u/wtf\textunderscore m1	,	&"	How is MLOps done in your current workplace?	",&	\url{	https://www.reddit.com/r/MachineLearning/comments/qk5avf/d_how_is_mlops_done_in_your_current_workplace/	},&		2021.
\smallskip \item
u/tchiotludo	,	&"	How Leroy Merlin managed their cloud data pipelines with Kestra	",&	\url{	https://www.reddit.com/r/dataengineering/comments/t8z5o9/how_leroy_merlin_managed_their_cloud_data/	},&		2022.
\smallskip \item
Louis Dorard	,	&"	How predictive APIs are used to Upwork Microsoft and BigML (and how they could be standardized)	",&	\url{	https://medium.com/papis-stories/how-predictive-apis-are-used-at-upwork-microsoft-and-bigml-and-how-they-could-be-standardized-2daaeb527d34	},&		2016.
\smallskip \item
Picsellia	,	&"	How to apply MLOps to Computer Vision? Introducing CVOps	",&	\url{	https://www.picsellia.com/post/how-to-apply-mlops-to-computer-vision-cvops	}	,&		2022.
\smallskip \item
Eckerson Group	,	&"	How to do DataOps with Snowflake: Tools and Rules - YouTube	",&	\url{	https://www.youtube.com/watch?v=AclviYOvClU	},&		2021.
\smallskip \item
K. Leung	,	&"	How to Dockerize Machine Learning Applications Built with H2O, MLflow, FastAPI, and Streamlit	",&	\url{	https://towardsdatascience.com/how-to-dockerize-machine-learning-applications-built-with-h2o-mlflow-fastapi-and-streamlit-a56221035eb5	},&		2022.
\smallskip \item
T.-I. Lasn	,	&"	How To Setup Continuous Integration (CI) With React, CircleCI, and GitHub	",&	\url{	https://medium.com/better-programming/how-to-setup-continuous-integration-ci-with-react-circleci-and-github-e0efd5040b03	},&		2019.
\smallskip \item
u/StorageReview\textunderscore Adam\textunderscore a	,	&"	HPE Ezmeral Introduced	",&	\url{	https://www.reddit.com/r/StorageReview/comments/heg8i5/hpe_ezmeral_introduced/	},&		2020.
\smallskip \item
HPE	,	&"	HPE Ezmeral ML Ops - Machine Learning Operations Software	",&	\url{	https://www.hpe.com/us/en/solutions/ezmeral-machine-learning-operations.html	},&	Accessed 2023.
\smallskip \item
u/alessya	,	&"	I am Alessya Visnjic, co-founder and CEO of WhyLabs. I am here to talk about MLOps, AI Observability and our recent product announcements. Ask me anything!	",&	\url{	https://www.reddit.com/r/mlops/comments/qrtszx/i_am_alessya_visnjic_cofounder_and_ceo_of_whylabs/	},&		2021.
\smallskip \item
u/erikvdplas	,	&"	Idea: MLOps Composer. Interested in the community's opinion! [Project]	",&	\url{	https://www.reddit.com/r/MachineLearning/comments/clx5sy/idea_mlops_composer_interested_in_the_communitys/	},&		2019.
\smallskip \item
Cometml	,	&"	If you \#ML code is part of your application codebase, you'll have to run an entire CI/CD pipeline each time you want to run another modeling experiment (likely many, many times). We're partnering with @gitlab to help solve this \#MLOps challenge.  https://t.co/9yi5vwll2k https://t.co/3NFDc95cEv	",&	\url{	https://twitter.com/Cometml/status/1459223721470791684	},&		2021.
\smallskip \item
D. Erb	,	&"	Improve MLOps and Accelerate Model Deployment with ...	",&	\url{	https://builders.intel.com/docs/aibuilders/improve-mlops-and-accelerate-model-deployment-with-paperspace-and-intel.pdf	},&		2021.
\smallskip \item
sbreddy2021	,	&"	Intelligent machine learning model deployment and consume pipeline with DataRobot AI cloud platform “MLOps”.  Cover in-depth details about the model deployment, model registry, model inference application.  https://t.co/a9dj1IY2C9	",&	\url{	https://twitter.com/sbreddy2021/status/1503402635491086337	},&		2022.
\smallskip \item
Armand Ruiz	,	&"	Introducing IBM Watson Studio	",&	\url{	https://medium.com/ibm-watson/introducing-ibm-watson-studio-e93638f0bb47	},&		2018.
\smallskip \item
u/eemamedo	,	&"	Is it possible to automatically deploy a ML pipeline to Airflow?	",&	\url{	https://www.reddit.com/r/mlops/comments/vzhsp0/is_it_possible_to_automatically_deploy_a_ml/	},&		2022.
\smallskip \item
Grigory Sapunov	,	&"	JAX Ecosystem	",&	\url{	https://medium.com/@moocaholic/jax-a13e83f49897	},&		2020.
\smallskip \item
Jina	,	&"	Jina AI: MLOps for Multimodal AI, Neural Search, Generative ...	",&	\url{	https://jina.ai/	},&	Accessed 2023.
\smallskip \item
u/Dazzling\textunderscore Koala6834	,	&"	Jira for ML tool	",&	\url{	https://www.reddit.com/r/jira/comments/zkngyw/jira_for_ml_tool/	},&		2022.
\smallskip \item
AiKatonic	,	&"	Katonic MLOPs platform is a native Kubernetes application, which reflects the strengths of the open-source container orchestration system: flexibility, reliability and avoiding vendor or tool lock-in. https://t.co/D8NDdSwbMo	",&	\url{	https://twitter.com/AiKatonic/status/1407524338257907715	},&		2021.
\smallskip \item
Ricardo Raspini Motta	,	&"	Kedro vs ZenML vs Metaflow: Which Pipeline Orchestration Tool Should You Choose?	",&	\url{	https://ricardormotta.medium.com/kedro-vs-zenml-vs-metaflow-which-pipeline-orchestration-tool-should-you-choose-1d52bfa56a5e	},&		2022.
\smallskip \item
Kili Technologies	,	&"	Kili Technology - Labeling Platform for High-Quality Training ...	",&	\url{	https://kili-technology.com/	}	,&	Accessed 2023.
\smallskip \item
Marnixvdb	,	&"	Launching our ML platform (or MLOps tool if we go with the times). See: https://t.co/B7VtupKVur. It has a pretty cool way of interacting with user code.	",&	\url{	https://twitter.com/Marnixvdb/status/1315677608382787585	},&		2020.
\smallskip \item
Lenses	,	&"	Lenses.io: DataOps platform for Apache Kafka and Kubernetes	",&	\url{	https://lenses.io/	},&	Accessed 2023.
\smallskip \item
TrastRadius	,	&"	List of Top MLOps Tools 2023 - TrustRadius	",&	\url{	https://www.trustradius.com/mlops	},&	Accessed 2023.
\smallskip \item
u/GTechLearn	,	&"	Machine Learning	",&	\url{	https://www.reddit.com/user/GTechLearn/comments/ys6k7a/machine_learning/	},&		2022.
\smallskip \item
D ONE	,	&"	Machine learning for production - introducing D ONE's MLOps ...	",&	\url{	https://d-one.ai/news/ml-ops	},&		2022.
\smallskip \item
K. Pham	,	&"	Machine Learning in iOS: IBM Watson and CoreML	",&	\url{	https://medium.com/flawless-app-stories/detecting-avengers-superheroes-in-your-ios-app-with-ibm-watson-and-coreml-fe38e493a4d1	},&		2018.
\smallskip \item
cnvrg.io	,	&"	Machine Learning Operations – MLOps - Cnvrg.io	",&	\url{	https://cnvrg.io/platform/mlops/	},&	Accessed 2023.
\smallskip \item
Microsoft	,	&"	Machine learning operations (MLOps) framework to upscale ...	",&	\url{	https://learn.microsoft.com/en-us/azure/architecture/example-scenario/mlops/mlops-technical-paper	},&	Accessed 2023.
\smallskip \item
Akira.AI	,	&"	Machine Learning Operations (MLOps) platform for Enterprises	",&	\url{	https://www.akira.ai/mlops-platform/	},&	Accessed 2023.
\smallskip \item
C. Y. Wijaya	,	&"	Manage ML Automation Workflow with DagsHub, GitHub Action, and CML	",&	\url{	https://medium.com/towards-artificial-intelligence/manage-ml-automation-workflow-with-dagshub-github-action-and-cml-a37fb50d5cb0	},&		2022.
\smallskip \item
A. Dhinakaran	,	&"	ML Infrastructure Tools for Model Building	",&	\url{	https://towardsdatascience.com/ml-infrastructure-tools-for-model-building-464770ac4fec	},&		2020.
\smallskip \item
Rapidminer	,	&"	ML Ops | Operationalize Your Models Faster - RapidMiner	",&	\url{	https://rapidminer.com/platform/ml-ops/	},&	Accessed 2023.
\smallskip \item
ankurkumarz	,	&"	MLflow - MLOps platform  OBS Studio - Video capture and live streaming Orange - data analysis \&amp; mining tool Pixie - observability tool for Kubernetes apps PostHog - instrumentation framework for product analytics	",&	\url{	https://twitter.com/ankurkumarz/status/1530740677981503489	},&		2022.
\smallskip \item
Pytorch	,	&"	MLflow and PyTorch — Where Cutting Edge AI meets MLOps	",&	\url{	https://medium.com/pytorch/mlflow-and-pytorch-where-cutting-edge-ai-meets-mlops-1985cf8aa789	},&		2020.
\smallskip \item
Databricks	,	&"	MLOps - Databricks	",&	\url{	https://www.databricks.com/glossary/mlops	},&	Accessed 2023.
\smallskip \item
DataRobot	,	&"	MLOps - DataRobot	",&	\url{	https://www.datarobot.com/platform/mlops/	},&	Accessed 2023.
\smallskip \item
AWS	,	&"	MLOps – Machine Learning Operations– Amazon Web Services	",&	\url{	https://aws.amazon.com/sagemaker/mlops/	},&	Accessed 2023.
\smallskip \item
u\ollie\textunderscore wollie\textunderscore rocks	,	&"	MLOps Community (recorded) session on new open source data prep tool	",&	\url{	https://www.reddit.com/r/MachineLearning/comments/w8ace0/d_mlops_community_recorded_session_on_new_open/	},&		2022.
\smallskip \item
trojrobert	,	&"	MLOps contain different components that are connected to form a pipeline.  How do we manage these components? A good tool for this is Kubeflow, kubeflow can be used to run components in a pipeline and automatically move from one step to another in the pipeline.  \#MLOps	",&	\url{	https://twitter.com/trojrobert/status/1465797612615999500	},&		2021.
\smallskip \item
arnabbiswas1	,	&"	MLOps friends, which tool to use to validate data in ML pipeline? 3 popular options: - GreatExpectations (@expectgreatdata) - TFX Data Validation  - AWS Deeque Any suggestion?  My simple pipeline uses pandas, joblib (for parallelization), airflow \&amp; resides in @Azure ecosystem	",&	\url{	https://twitter.com/arnabbiswas1/status/1466395947848507399	},&		2021.
\smallskip \item
T. Kaza	,	&"	MLOps Lifecycle - VivSoft	",&	\url{	https://www.vivsoft.io/post/mlops	}	,&		2020.
\smallskip \item
S. Abid	,	&"	MLOps Lifecycle: What are the stages of MLOps development	",&	\url{	https://www.bitstrapped.com/blog/mlops-lifecycle-explained-by-stages	},&		2022.
\smallskip \item
Google Cloud	,	&"	MLOps on Vertex AI | Google Cloud	",&	\url{	https://cloud.google.com/vertex-ai/docs/start/introduction-mlops	},&	Accessed 2023.
\smallskip \item
u/Shoddy\textunderscore Change\textunderscore 6559	,	&"	MLOps Perspective on Creating a Two-Layered Recommendation System	",&	\url{	https://www.reddit.com/r/mlops/comments/wj5o5k/mlops_perspective_on_creating_a_twolayered/	},&		2022.
\smallskip \item
Neuro	,	&"	MLOps platform | Neuro	",&	\url{	https://neu.ro/	},&	Accessed 2023.
\smallskip \item
u/krumb0y	,	&"	MLOps project based template	",&	\url{	https://www.reddit.com/r/mlops/comments/q60i5b/mlops_project_based_template/	},&		2021.
\smallskip \item
u/putinwhat	,	&"	MLOps Stack	",&	\url{	https://www.reddit.com/r/MachineLearning/comments/mtejw5/d_mlops_stack/	},&		2021.
\smallskip \item
u/sinohi	,	&"	MLops tool for image data management and exploration	",&	\url{	https://www.reddit.com/r/MachineLearning/comments/qoqp4w/discussion_mlops_tool_for_image_data_management/	},&		2021.
\smallskip \item
N. S. Gill	,	&"	MLOps Tools and its Processes | The Complete Guide	",&	\url{	https://www.xenonstack.com/blog/mlops-processes	},&		2022	.
\smallskip \item
M. Ali	,	&"	MLOps Tools and Technologies for Data Scientists in 2022	",&	\url{	https://moez-62905.medium.com/mlops-tools-and-technologies-for-data-scientists-in-2022-dc87659ae053	},&		2022.
\smallskip \item
Censius	,	&"	MLOps Tools for Machine Learning Lifecycle - Censius	",&	\url{	https://censius.ai/mlops-tools	},&	Accessed 2023.
\smallskip \item
S. Teki	,	&"	MLOps tools, MLOps tech stack - Sundeep Teki	",&	\url{	https://www.sundeepteki.org/blog/top-mlops-tools	},&		2022.
\smallskip \item
R. Cutting and K. Alscher	,	&"	MLOps Tools: The Ins and Outs of Choosing a Cloud Provider	",&	\url{	https://www.wwt.com/article/mlops-tools-the-ins-and-outs-of-choosing-cloud-provider	},&		2022.
\smallskip \item
Aporia team	,	&"	MLOps Toys | A Curated List of Machine Learning Projects	",&	\url{	https://mlops.toys/	},&		2021.
\smallskip \item
u/Panthums	,	&"	MLOps using IBM Cloud tools	",&	\url{	https://www.reddit.com/r/mlops/comments/r25aqi/mlops_using_ibm_cloud_tools/	},&		2021.
\smallskip \item
Softmax	,	&"	MLOps vs DevOps - SoftmaxAI	",&	\url{	https://softmaxai.com/mlops-vs-devops/	},&	Accessed 2023	.
\smallskip \item
F. Buso and J. Dowling	,	&"	MLOps with a Feature Store - Hopsworks	",&	\url{	https://www.hopsworks.ai/post/mlops-with-a-feature-store	},&		2020.
\smallskip \item
Dataiku	,	&"	MLOps with Dataiku	",&	\url{	https://www.dataiku.com/product/key-capabilities/mlops/	},&	Accessed 2023.
\smallskip \item
Pelin	,	&"	MLOps with Flyte: Between Machine Learning and Engineering	",&	\url{	https://mlops.community/mlops-with-flyte-the-convergence-of-workflows-between-machine-learning-and-engineering/	},&		2022.
\smallskip \item
A. Tripathi	,	&"	MLOps: A Complete Guide to Machine Learning Operations	",&	\url{	https://ashutoshtripathi.com/2021/08/18/mlops-a-complete-guide-to-machine-learning-operations-mlops-vs-devops/	},&		2021.
\smallskip \item
W. Pok	,	&"	MLOps: How to choose the best ML model tools | Blogs	",&	\url{	https://www.ambiata.com/blog/2020-12-07-mlops-tools/	},&		2020.
\smallskip \item
Altexsoft	,	&"	MLOps: Methods and Tools of DevOps for Machine Learning	",&	\url{	https://www.altexsoft.com/blog/mlops-methods-tools/	},&		2020.
\smallskip \item
M. Schmitt	,	&"	MLOps: the ultimate guide - Data Revenue	",&	\url{	https://www.datarevenue.com/en-blog/mlops-the-ultimate-guide	},&	Accessed 2023.
\smallskip \item
Iguazio	,	&"	MLRun: Open Source MLOps Orchestration	",&	\url{	https://www.mlrun.org/	},&	Accessed 2023	.
\smallskip \item
u/Last-Programmer2181	,	&"	Model Deployments / DS gitflow	",&	\url{	https://www.reddit.com/r/mlops/comments/ys0u5p/model_deployments_ds_gitflow/	}	,&		2022.
\smallskip \item
c3.ai	,	&"	Model Ops - C3 AI	",&	\url{	https://c3.ai/c3-ai-application-platform/ai-application-development/model-ops/	},&	Accessed 2023.
\smallskip \item
Gartner Peer Insights	,	&"	Multipersona Data Science and Machine Learning Platforms	",&	\url{	https://www.gartner.com/reviews/market/multipersona-data-science-and-machine-learning-platforms	},&	Accessed 2023.
\smallskip \item
T. Blogumas	,	&"	Must Learn DevOps Tools for 2020	",&	\url{	https://betterprogramming.pub/must-learn-devops-tools-for-2020-1a8a2675e88f	}	,&		2020.
\smallskip \item
T. Sarnet and N. Campos	,	&"	MyMLOps	",&	\url{	https://www.mymlops.com	},&		2022.
\smallskip \item
OpenJS Foundation	,	&"	Node-RED	",&	\url{	https://nodered.org/	},&	Accessed 2023.
\smallskip \item
O.Savsunenko	,	&"	Optimizing neural networks for production with Intel’s OpenVINO	",&	\url{	https://medium.com/hackernoon/optimizing-neural-networks-for-production-with-intels-openvino-a7ee3a6883d	},&		2018.
\smallskip \item
045\textunderscore hamid	,	&"	orchest is a very handy and useful tool for creating and building \#DataScience  pipelines. https://t.co/dGyzqXiYmo \#MLOps \#MachineLearning  \#opensource \#DevOps \#sysadmin \#SRE \#Linux \#coding \#FOSS \#freesoftware \#programming \#Python \#docker \#pipeline  https://t.co/6GjGhLsp4K	",&	\url{	https://twitter.com/045_hamid/status/1478662513789124616	},&		2022.
\smallskip \item
K. Tran	,	&"	Orchestrate a Data Science Project in Python With Prefect	",&	\url{	https://medium.com/towards-data-science/orchestrate-a-data-science-project-in-python-with-prefect-e69c61a49074	},&		2021.
\smallskip \item
Netflix Technology Blog	,	&"	Orchestrating Data/ML Workflows at Scale With Netflix Maestro	",&	\url{	https://netflixtechblog.com/orchestrating-data-ml-workflows-at-scale-with-netflix-maestro-aaa2b41b800c	},&		2022.
\smallskip \item
Polyaxon	,	&"	Polyaxon: Open source Machine Learning at scale with ...	",&	\url{	https://polyaxon.com/	},&	Accessed 2023.
\smallskip \item
D. Radečić	,	&"	Prefect: How to Write and Schedule Your First ETL Pipeline with Python	",&	\url{	https://medium.com/towards-data-science/prefect-how-to-write-and-schedule-your-first-etl-pipeline-with-python-54005a34f10b	},&		2021.
\smallskip \item
u/badge	,	&"	Recommended ML Ops tools for \textunderscore tiny\textunderscore  models	",&	\url{	https://www.reddit.com/r/datascience/comments/q2rrqh/recommended_ml_ops_tools_for_tiny_models/	},&		2021.
\smallskip \item
R. Mohanan	,	&"	Review: AWS SageMaker vs. Azure ML: Which MLOps ...	",&	\url{	https://www.spiceworks.com/tech/innovation/articles/aws-sagemaker-vs-azure-ml-review/	},&		2022.
\smallskip \item
Rivery	,	&"	Rivery: Cloud ELT Tool | Data Pipeline \& Integration Platform	",&	\url{	https://rivery.io/	},&	Accessed 2023.
\smallskip \item
DrMattCrowson	,	&"	RT Under appreciated workflow tool — Airflow https://t.co/W9mxKDDcGG \#machinelearning \#python \#mlops \#airflow \#workflow https://t.co/nN1Qb3SEZK	",&	\url{	https://twitter.com/DrMattCrowson/status/1397248256883650560	},&		2021.
\smallskip \item
run:ai	,	&"	Run:ai - AI Optimization and Orchestration	",&	\url{	https://www.run.ai/	},&	Accessed 2023.
\smallskip \item
Ryax Technologies 	,	&"	Ryax, the DataOps platform for business analysts	",&	\url{	https://ryax.tech/product/	},&	Accessed 2023.
\smallskip \item
DataRobot	,	&"	See how to integrate @ApacheAirflow, a popular open source orchestration tool and workflow scheduler, into your DataRobot orchestration and MLOps workflows. https://t.co/PSDsr2ceG5	",&	\url{	https://twitter.com/DataRobot/status/1537537258076745733	},&		2022.
\smallskip \item
Seldon Technologies	,	&"	Seldon, MLOps for the Enterprise.	",&	\url{	https://www.seldon.io/	},&	Accessed 2023.
\smallskip \item
u/[deleted]	,	&"	Self-hosting tools for ML ops/experiment management (e.g. wandb or kubeflow)	",&	\url{	https://www.reddit.com/r/selfhosted/comments/uj6k3o/selfhosting_tools_for_ml_opsexperiment_management/	},&		2022.
\smallskip \item
u/neutralino	,	&"	Sematic – an open-source ML pipelining tool built by ex-Cruise engineers	",&	\url{	https://www.reddit.com/r/mlops/comments/z9sjmw/sematic_an_opensource_ml_pipelining_tool_built_by/	},&		2022.
\smallskip \item
u/FrazerNg	,	&"	Should I transition from MLE to DE? Rant/experience sharing from a 2 YOE MLE with imposter syndrome	",&	\url{	https://www.reddit.com/r/datascience/comments/vhc8ei/should_i_transition_from_mle_to_de_rantexperience/	},&		2022.
\smallskip \item
Streamlit	,	&"	Streamlit • The fastest way to build and share data apps	",&	\url{	https://streamlit.io/	},&	Accessed 2023.
\smallskip \item
StreamSets	,	&"	StreamSets: Data Integration Platform for Enterprise Companies	",&	\url{	https://streamsets.com/	},&	Accessed 2023.
\smallskip \item
EvidentlyAI	,	&"	Taking models from prototype to production was a challenge. @Grubhub ML team built a platform to scale it. Modular architecture:   data access objects shared feature pool  application layer utility libraries  \#MLOps details  https://t.co/03sEQAUD8Z	",&	\url{	https://twitter.com/EvidentlyAI/status/1316355071022596098	},&		2020.
\smallskip \item
Tensorflow	,	&"	TensorFlow	",&	\url{	https://www.tensorflow.org/	},&	Accessed 2023.
\smallskip \item
T. King	,	&"	The 16 Best Data Science Software and Machine Learning ...	",&	\url{	https://solutionsreview.com/business-intelligence/the-best-data-science-and-machine-learning-platforms/	},&		2022.
\smallskip \item
Jakub Czakon	,	&"	The Best MLOps Tools and How to Evaluate Them	",&	\url{	https://neptune.ai/blog/best-mlops-tools	}	,&		2022.
\smallskip \item
Delphix	,	&"	The Delphix DevOps Data Platform	",&	\url{	https://www.delphix.com/platform	},&	Accessed 2023.
\smallskip \item
clearmlapp	,	&"	The meta-question here is the following: In a world where you can get decent autogenerated code for your ML pipeline, and you also wish to integrate an MLOps tool on top of it, is it flexible enough? Or, as we say, could you "build your own on top?"	",&	\url{	https://twitter.com/clearmlapp/status/1419643691124203520	},&		2021.
\smallskip \item
R. Romano	,	&"	The ultimate guide to MLOps tools in 2022 | Qwak's Blog	",&	\url{	https://www.qwak.com/post/the-ultimate-guide-to-mlops-tools-in-2022	},&		2022.
\smallskip \item
sanjaykalra	,	&"	There are multiple \#MLOps tools for each part of the pipeline, and we see a world where each tool has enough market space to support it becoming a large company.  @insightpartners \#MachineLearning  https://t.co/SNxEljikoa https://t.co/YgbwppQyjo	",&	\url{	https://twitter.com/sanjaykalra/status/1493398132406685699	},&		2022.
\smallskip \item
u/asadfaizi	,	&"	Tools to start Machine Learning Using Docker and Kubernetes	",&	\url{	https://www.reddit.com/r/kubernetes/comments/pcw616/tools_to_start_machine_learning_using_docker_and/	},&		2021.
\smallskip \item
Iconiq Inc.	,	&"	Top 10 MLOps Tools to Learn in 2023 - ProjectPro	",&	\url{	https://www.projectpro.io/article/best-mlops-tools-/574	},&	Accessed 2023	.
\smallskip \item
S. Bellamkonda	,	&"	Top 10 MLOps Tools to Optimize \& Manage Machine Learning ...	",&	\url{	https://www.kdnuggets.com/2022/10/top-10-mlops-tools-optimize-manage-machine-learning-lifecycle.html	},&		2022.
\smallskip \item
The Chief I/O	,	&"	Top 10 Open Source MLOps Tools	",&	\url{	https://thechief.io/c/editorial/top-10-open-source-mlops-tools/	},&	Accessed 2023.
\smallskip \item
M. Trends	,	&"	Top 10 Open-Source MLOps Tools Every Software Developer ...	",&	\url{	https://www.analyticsinsight.net/top-10-open-source-mlops-tools-every-software-developer-should-know/	},&		2022.
\smallskip \item
SWAPNANJAN K	,	&"	Top 20 DataOps Tools and Its Ranking in 2023	",&	\url{	https://www.devopsschool.com/blog/top-20-dataops-tools-and-its-ranking/	},&		2022.
\smallskip \item
S. Singh	,	&"	Top 5 Tools for MLOps - LinkedIn	",&	\url{	https://www.linkedin.com/pulse/top-5-tools-mlops-sreeshti-singh?trk=pulse-article_more-articles_related-content-card	},&		2022.
\smallskip \item
u/ai-lover	,	&"	Top Dataops Tools/Platforms in 2022	",&	\url{	https://www.reddit.com/r/machinelearningnews/comments/yxio3p/top_dataops_toolsplatforms_in_2022/	},&		2022.
\smallskip \item
u/ai-lover	,	&"	Top MLOps Platforms/Tools to Manage the Machine Learning Lifecycle in 2022	",&	\url{	https://www.reddit.com/r/MLOPSNEWS/comments/xwu71e/top_mlops_platformstools_to_manage_the_machine/	},&		2022.
\smallskip \item
T. Papapanagiotou	,	&"	Towards MLOps: technical capabilities of a machine learning ...	",&	\url{	https://www.prosus.com/news/towards-mlops-technical-capabilities-of-a-machine-learning-platform/	},&		2021.
\smallskip \item
u/UBIAI	,	&"	Traditional pipeline and advanced MLOps	",&	\url{	https://www.reddit.com/user/UBIAI/comments/xcno49/traditional_pipeline_and_advanced_mlops/	},&		2022.
\smallskip \item
u/htahir1	,	&"	Tutorial: Serverless MLOps pipelines with Vertex AI and ZenML	",&	\url{	https://www.reddit.com/r/MachineLearning/comments/vsufhh/p_tutorial_serverless_mlops_pipelines_with_vertex/	},&		2022.
\smallskip \item
Vimarsh Karbhari	,	&"	Uber’s Michaelangelo — ML Platform	",&	\url{	https://medium.com/acing-ai/ubers-michaelangelo-ml-platform-77d03d8cbe57	},&		2021.
\smallskip \item
valohaiai	,	&"	Valohai | Take ML places it's never been	",&	\url{	https://valohai.com/	},&	Accessed 2023.
\smallskip \item
Verta	,	&"	Verta | Model Management \& Operations for MLOps and ...	",&	\url{	https://www.verta.ai/	},&	Accessed 2023.
\smallskip \item
u/modzykirsten	,	&"	Video: MLOps \& CI/CD	",&	\url{	https://www.reddit.com/r/developers/comments/wmp9za/video_mlops_cicd/	},&		2022.
\smallskip \item
StartupBoomer	,	&"	Watch the story of @hasty\textunderscore ai and learn how their AI-Driven Image Annotation Software Platform, can be useful for your enterprise to go from raw images or videos to production-ready model in one tool. No MLops skills or tricky integrations needed. \#Germany https://t.co/X79NYmXYWV	",&	\url{	https://twitter.com/StartupBoomer/status/1432725466083889164	},&		2021.
\smallskip \item
Qwak\textunderscore ai	,	&"	We are so happy to be identified by @hackernoon as the top platform and tool for Machine Learning (MLOps)Learn more about MLOps in the article: https://t.co/f8PxS0vSSu \#machinelearning \#ML	",&	\url{	https://twitter.com/Qwak_ai/status/1526964950215933952	},&		2022.
\smallskip \item
Weights \& Biases	,	&"	Weights \& Biases – Developer tools for ML	",&	\url{	https://wandb.ai/site	},&	Accessed 2023.
\smallskip \item
Apache Software Foundation	,	&"	Welcome | Superset	",&	\url{	https://superset.apache.org/	},&	Accessed 2023.
\smallskip \item
Alteryx	,	&"	What Is MLOps? | Alteryx	",&	\url{	https://www.alteryx.com/glossary/mlops	},&	Accessed 2023.
\smallskip \item
F. Knuper	,	&"	What is MLOps? | New Relic	",&	\url{	https://newrelic.com/blog/best-practices/what-is-mlops	},&		2021.
\smallskip \item
u/fripperML	,	&"	What’s the simplest, most lightweight but complete and 100\% open source MLOps toolkit?	",&	\url{	https://www.reddit.com/r/MachineLearning/comments/mfca0p/d_whats_the_simplest_most_lightweight_but/	},&		2021.
\smallskip \item
pachyderminc	,	&"	When it comes to MLOps, no one tool can do it all. It takes an array of best-of-breed tools to truly automate the entire ML lifecycle. This post will cover the \#MLOps Ecosystem and @pachyderminc solutions: https://t.co/4vmCfvRnWq  \#ai \#datacentricai \#machinelearning  \#data \#IoT https://t.co/LrDMWKZ2eX	",&	\url{	https://twitter.com/pachyderminc/status/1577309794523815936	},&		2022.
\smallskip \item
neptune\textunderscore ai	,	&"	When it’s not recommended 2:  You already use a tool that could be used for MLOps. E.g. you use Apache Airflow for ETL processes -\&gt; Probably makes more sense to use this tool for MLOps rather than building an MLOps pipeline with GitHub.	",&	\url{	https://twitter.com/neptune_ai/status/1503327882000617476	},&		2022.
\smallskip \item
OHamzaoui1	,	&"	When researching what tool(s) to adopt for an ML platform, you certainly came across a tooling landscape picture like the one below.Before zooming in, check out the article "MLOps Is a Mess But That's to be Expected" by @mihail\textunderscore eric.: https://t.co/5ToGhY58ik \#MLOps  \#AI https://t.co/33Tmavoq0v	",&	\url{	https://twitter.com/OHamzaoui1/status/1511027251177000962	},&		2022.
\smallskip \item
u/mrcet007	,	&"	Which is the best tool for creating continuous training pipelines for MLOPS ?	",&	\url{	https://www.reddit.com/r/datascience/comments/q9e7jg/which_is_the_best_tool_for_creating_continuous/	},&		2021.
\smallskip \item
u/zedrakk	,	&"	Would an ML Ops platform be useful?	",&	\url{	https://www.reddit.com/r/MachineLearning/comments/uhauw5/d_would_an_ml_ops_platform_be_useful/	},&		2022.
\smallskip \item
kargarisaac	,	&"	You can also easily add different \#MLOps tools to your stack. In this blog post, I show how to create the stack and run your pipeline on \#VertexAI on \#GCP with \#MLflow as an experiment tracker. In the next blog post, I will go over adding a model deployment tool to the stack.	",&	\url{	https://twitter.com/kargarisaac/status/1565627175415472128	},&		2022.
\smallskip \item
ZenML	,	&"	ZenML Home	",&	\url{	https://zenml.io/home	},&	Accessed 2023.
\smallskip \item
u/benkoller	,	&"	ZenML Open-Source MLOps - Plus: Feature Expectations	",&	\url{	https://www.reddit.com/r/MachineLearning/comments/khljmi/p_zenml_opensource_mlops_plus_feature_expectations/	},&		2020.
\smallskip \item
u/htahir1	,	&"	ZenML: An extensible, open-source framework to create reproducible machine learning pipelines	",&	\url{	https://www.reddit.com/r/MachineLearning/comments/rgcrfj/p_zenml_an_extensible_opensource_framework_to/	},&		2021.
\smallskip\item
u/htahir2	,	&"	ZenML: Build vendor-agnostic, production-ready MLOps pipelines	",&	\url{	https://www.reddit.com/r/MachineLearning/comments/uxl8ds/p_zenml_build_vendoragnostic_productionready/	},&		2021.
\end{enumerate}
